# Supplementary material for: Combinatorial decompositions for deformed or decorated classes of maps
Source: arXiv:2312.00056 source file (2023-11-29)
Supplement: Supplementary file 1 [file AppendixTemplate.tex]

% Appendix Template

\chapter{Appendix Title Here} % Main appendix title
\label{AppendixX} % Change X to a consecutive letter; for referencing this appendix elsewhere, use \ref{AppendixX}

Write your Appendix content here.
